# Supplementary material for: Robot Synesthesia: In-Hand Manipulation with Visuotactile Sensing
Source: arXiv:2312.01853 source file (2024-07-31)
Supplement: Supplementary file 1 [file supp.tex]

\subsection{Training Hyper-parameters}
Table \ref{tab:exp:rew_hyperparam} lists the hyper-parameters for our reward function shown in equation \ref{rew-equation}. Once the distance between the object and the hand center reaches the fall distance, we add a fall penalty of 50 to the reward function.

We train our teacher policy with PPO, and the training hyper-parameters are shown in Table \ref{tab:exp:ppo_hyperparam}. Specifically, we train with 8192 parallel environments. Each environment gathers \# steps data to train in each epoch of PPO. The data is split into \# minibatches and optimized with PPO loss. $\gamma$ and $\lambda$ are used for computing generalized advantage estimate (GAE) returns. We use Adam optimizer and adaptive learning rate to train PPO, and adopt the gradient clip to stabilize training. We train 4000 epochs in total, which takes less than one day on a single GPU. We train student policies with BC and DAgger, and the hyper-parameters are shown in Table \ref{tab:exp:bc_hyperparam}.

\begin{table}[]
    \centering
    \caption{Hyper-parameters for the reward function. }
    \begin{tabular}{ll}
        \toprule
        Hyper-parameters     & Values \\
        \midrule
        $c_1$ & 1.0 \\
        $c_2$ & -0.1 \\
        $c_3$ & 0.1 \\
        $c_4$ & -0.0003 \\
        $c_5$ & -0.0003 \\
        $c_6$ & 0.0 \\
        fall distance & 0.1 \\
        fall penalty & 50.0 \\
        \bottomrule
    \end{tabular}
    \label{tab:exp:rew_hyperparam}
    
\end{table}

\begin{table}[]
    \centering
    \caption{Hyper-parameters for training teacher policies.}
    \begin{tabular}{llllllll}
        \toprule
        Hyper-parameters     & Values \\
        \midrule
        \# environments & 8192 \\
        \# steps             & 16  \\
        \# minibatches       & 16384     \\
        \# epochs & 4000 \\
        $\gamma$                & 0.99   \\
        $\lambda$                  & 0.95   \\
        learning rate       & 1e-4 \\
        clip range          & 0.2    \\
        entropy coefficient            & 0.0   \\
        critic coefficient & 5.0 \\
        kl threshold & 0.02 \\
        max gradient norm      & 1.0    \\
        \bottomrule
    \end{tabular}
    \label{tab:exp:ppo_hyperparam}
    \vspace{-5mm}
\end{table}

\begin{table}[]
    \centering
    \caption{Hyper-parameters for training student policies.}
    \begin{tabular}{llllllll}
        \toprule
        Hyper-parameters     & Values \\
        \midrule
        \# environments & 64 \\
        \# steps             & 200  \\
        \# minibatches       & 1024     \\
        \# epochs & 400 \\
        learning rate       & 5e-5 \\
        \bottomrule
    \end{tabular}
    \label{tab:exp:bc_hyperparam}
\end{table}

\subsection{More Results on Double-ball Rotation}
We further evaluate our double-ball policy on different sets of real-world balls, shown in Table~\ref{Table:real-eval-ball} and Figure~\ref{fig:two-ball}. As the real-world balls we test on vary significantly in weight, density, size and texture, our policy generalizes well to novel objects and behaves more robustly compared with baselines.

\begin{table*}[h]
\centering
\caption{Evaluation of our double-ball policy (CRA/TTF) on different sets of real-world balls. Each policy is tested for 5 episodes. Each trial lasts 60 seconds.}
\begin{tabular}{ccccccccccccccccccc}
\toprule[1pt]
Obs Type &  \\
(CRA/TTF)& \multirow{-2}{*}{Two Tomatoes} &   \multirow{-2}{*}{Two Potatoes}& \multirow{-2}{*}{Two Golfballs} & \multirow{-2}{*}{Golfball-Tomato} & \multirow{-2}{*}{Golfball-Potato} &  \multirow{-2}{*}{Tomato-Potato}\\
\midrule[0.5pt]
Touch & 11.6/20.8 & 9.2/23.0 &  29.8/41.6 & 35.4/50.2 & 6.8/23.2 &  7.4/17.0  \\ 
Cam+Aug & 9.2/22.4 & 9.2/22.8 &  16.6/25.8 & 13.8/29.6 & 8.0/17.0 &  5.6/16.2\\
Touch+Cam+Aug & 18.6/31.2 & 6.6/15.0 &  35.0/51.0 & 32.0/53.0 & \textbf{22.8/41.4} &  9.4/26.8 \\
Touch+Cam+Aug+Syn & \textbf{24.2/40.0} & \textbf{22.4/42.0} &  \textbf{41.6/60.0} &  \textbf{42.0/60.0} & 8.2/16.2 &  \textbf{9.8/21.0}  \\ \bottomrule[1pt]
\end{tabular}
\label{Table:real-eval-ball}
% \vspace{-5mm}
\end{table*}

\begin{figure*}[h]
    \centering
    \includegraphics[width=\linewidth]{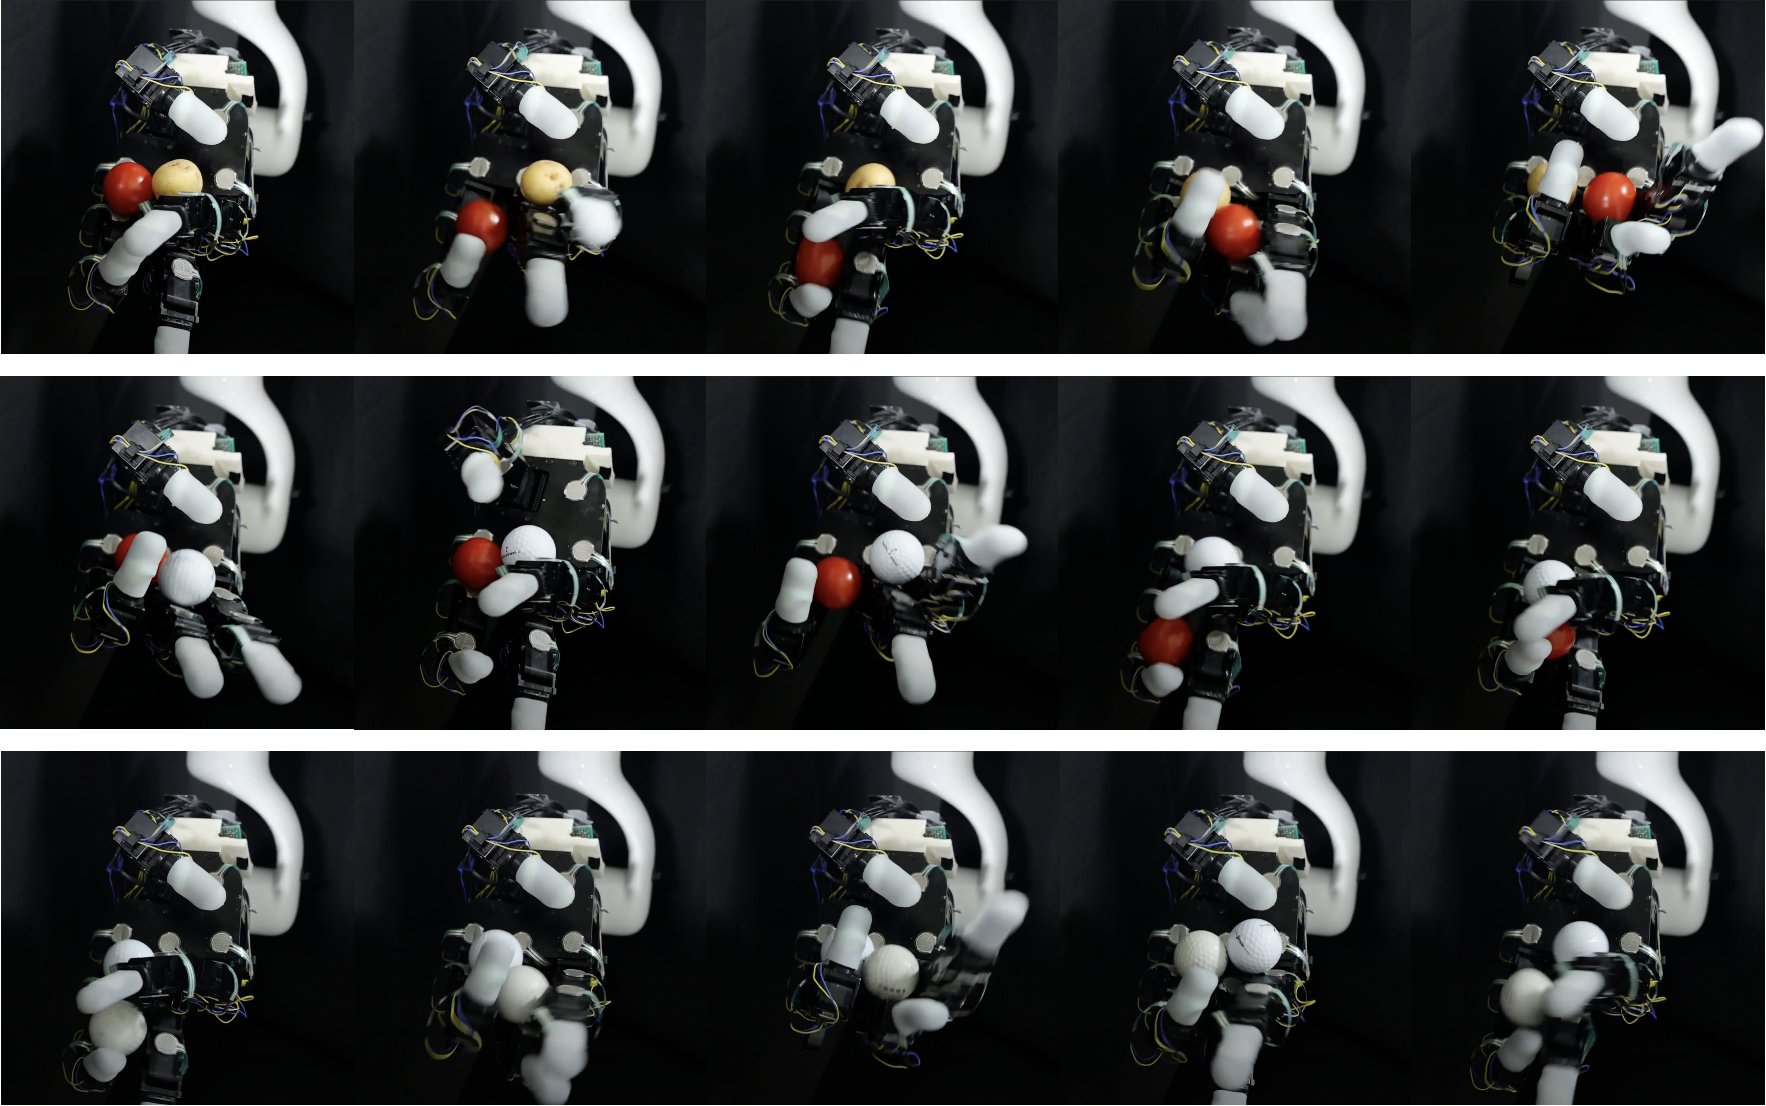}
    \caption{Visualization of our double-ball policy in the real-world testing on Tomato-Potato, Golfball-Tomato, and Two Golfballs.
    }
    \label{fig:two-ball}
    \vspace{-5mm}
\end{figure*}

%\subsection{More Discussion on Baselines}
